# Supplementary material for: The computation of approximate feedback Stackelberg equilibria in multi-player nonlinear constrained dynamic games
Source: arXiv:2401.15745 source file (2025-04-02)
Supplement: Supplementary file 1 [file appendix_kkt.tex]

\subsection{KKT conditions for two-player LQ games}\label{appendix:KKT}
The KKT condition for player 2 at the terminal time can be formulated as
% \begin{equation}
%     \begin{aligned}
%         \begin{bmatrix}
%             R_T^{2,2,2} & 0 & -G_{u_T^2}^{2\top} & -H_{u_T^2}^{2\top} & \hat{B}_T^{2\top} & 0 \\
%             0 & \hat{\gamma}_{T:T+1}^2 & \hat{s}_{T:T+1,k} & 0 &0 &0 \\
%             G_{u_T^2}^2 & -I &0 &0&0&0\\
%             H_{u_T^2}^2 & 0 & &0&0&0\\
%             -B_T^2 & 0 &0 &0 &0 &I \\
%             0 &0&0&0&-I&Q_{T+1}^2
%         \end{bmatrix}
%     \end{aligned}
% \end{equation}
\begin{equation*}\small
    \begin{aligned}
        &\begin{bmatrix}
            {R_T^{2,2,2}}&0&-G_{u_T^2}^{2\top}&-H_{u_T^{2}}^{2\top} & B_T^{2\top}&0&0&0&0 \\
            0 &\hat{\gamma}_{T}^2 & \hat{s}_{T}^2 &0&0&0&0&0&0\\
            G_{u_T^2}^2 & -I & 0 & 0 &0 &0 &0 &0 &0\\
            H_{u_T^2}^2 &0 & 0 & 0 &0& 0 & 0 &0 &0\\
            -B_T^2&0 &0& 0 & 0 & I & 0 &0&0 \\
            0&0 &0& 0 &-I & Q_{T+1}^2  &0 & - G_{x_{T+1}}^{2\top} & {-H_{x_{T+1}}^{2\top}} \\
            0&0&0&0&0&0&\hat{\gamma}_{T+1}^2 &\hat{s}_{T+1}^2 &0\\
            0&0 &0& 0 & 0 &G_{x_{T+1}}^2  & -I &0 &0 \\
            0&0 &0 &0 &0 & H^2_{x_{T+1}}& 0 &0 &0
        \end{bmatrix}
          \\& \cdot \begin{bmatrix}
            \Delta u_T^2\\ \Delta s_T^2 \\ \gamma_T^2 \\ \mu_T^2 \\ \lambda_T^2 \\ \Delta x_{T+1}  \\ \Delta s_{T+1}^2 \\ \gamma_{T+1}^2 \\ \mu_{T+1}^2
        \end{bmatrix} + \begin{bmatrix}
            {S_t^{2,2}} & {R_t^{2,2,1}}\\
            0 & 0 \\
            G_{x_T}^2 &  G_{u_{T}^1}^2 \\
            H^2_{x_T} & H^2_{u_T^1}\\
            -A_T & -B_T^1\\
            0 & 0 \\ 
            0 & 0 \\
            0 & 0 \\
            0 & 0
        \end{bmatrix} 
        \begin{bmatrix}
            \Delta x_T \\ \Delta u_T^1
        \end{bmatrix}+ \begin{bmatrix}
            r_T^2 \\ %\hat{\gamma}_{T,k}^2s_{T,k}^2 
            - \rho \mathbf{1}\\ g_{T,k}^2-s_{T,k}^2 \\ h_T^2\\ -c_T \\ q_{T+1}^2 \\ %\hat{\gamma}_{T+1,k}^2 s_{T+1,k}^2 
            - \rho\mathbf{1} \\ g_{T+1,k}^2 - s_{T+1,k}^2 \\ h_{T+1}^2
            % \\
            % \hat{\gamma}_{T,k}^2 g_{T,k}^2 - \frac{1}{t} \mathbf{1}
        \end{bmatrix} = 0
    \end{aligned}
\end{equation*}
where $\hat{\gamma}_t = $
We derive $\nabla \pi_T^2$ as in \eqref{eq:T,N,policy gradient}, and use it to construct leader's KKT condition:
% \begin{equation}\small
%     \begin{aligned}
%         \begin{bmatrix}
%             R_{T}^{1,1,1} & 0 & -G_{u_T^1}^{1\top} & -H_{u_T^1}^{1\top} & B_T^{1\top} & 0 & 0 & 0 & 0 \\
%             0 & \hat{\gamma}_T^1 & \hat{s}_{T}^1 & 0 & 0 &0&0&0&0 \\
%             G_{u_T^1}^1 & -I & 0 & 0 & 0 &0&0&0&0\\
%             H_{u_T^1}^1 & 0 &0&0&0&0 &0&0&0\\
%             -B_T^1&0 &0& 0 & 0 & I & 0 &0&0 \\
%             0&0 &0& 0 &-I & Q_{T+1}^2  &0 & - G_{x_{T+1}}^{2\top} & {-H_{x_{T+1}}^{2\top}} \\
%             0&0&0&0&0&0&\hat{\gamma}_{T+1,k}^2 &\hat{s}_{T+1,k}^2 &0\\
%             0&0 &0& 0 & 0 &G_{x_{T+1}}^2  & -I &0 &0 \\
%             0&0 &0 &0 &0 & H^2_{x_{T+1}}& 0 &0 &0
%         \end{bmatrix}
%         \begin{bmatrix}
%             \Delta u_T^1 \\ \Delta s_T^1 \\ \gamma_T^1 \\ \mu_T^1 \\ \lambda_T^1 \\ \Delta s_{T+1}^1 \\ \gamma_{T+1}^1 \\ \mu_{T+1}^1
%         \end{bmatrix}
%     \end{aligned}
% \end{equation}
\begin{equation*}\small
    \begin{aligned}
        &\begin{bmatrix}
            {R_T} &0 & -\hat{G}_{u_T}^\top& -\hat{H}_{u_T}^\top & \hat{B}_T^\top & {\Pi_T^{2\top}}&0&0&0&0 \\ 
            0 & \hat{\gamma}_{T} & \hat{s}_{T} &0&0&0&0&0&0&0 \\
            G_{u_T} & -I &0 &0&0 &0&0 &0 &0&0\\
            H_{u_T}&0 & 0 & 0 & 0 & 0 & 0 &0&0&0 \\
            -B_T&0&0 & 0 & 0 &  0 &  I_n  & 0 &0&0\\
            0&0&0 & 0 & -I_{2n} & 0 & Q_{T+1} &0 & -\hat{G}_{x_{T+1}}^\top & -\hat{H}_{x_{T+1}}^\top   \\
            0&0&0&0&0&0&0&\hat{\gamma}_{T+1} & \hat{s}_{T+1} &0\\
            0&0&0 & 0 & 0 & 0& G_{x_{T+1}} & -I &0&0  \\
            0&0 &0 &0 &0 &0  & H_{x_{T+1}} &0 &0&0 \\
            {\tilde{R}_T^{12}}&0 &-\tilde{G}_{u_T}^{12\top}& -\tilde{H}_{u_T}^{12\top} & \tilde{B}_T^{2\top} & -I_{m_2} & 0 & 0 &0&0\end{bmatrix} \\ &\cdot \begin{bmatrix}
            \Delta u_T \\ \Delta s_T \\ \gamma_T \\ \mu_T \\ \lambda_T \\ \psi_T^1 \\ \Delta x_{T+1} \\ \Delta s_{T+1} \\ \gamma_{T+1} \\ \mu_{T+1} 
        \end{bmatrix} + \begin{bmatrix}
            {S_{x_T}} \\ 0 \\ G_{x_T}  \\ H_{x_T} \\ -A_T \\ 0 \\ 0 \\ 0 \\ 0 \\ S_{T}^{12}
        \end{bmatrix}\Delta x_T + \begin{bmatrix}
            r_T \\ %\hat{\gamma}_{T,k}s_{T,k}
            -\rho\mathbf{1} \\ g_{T,k} - s_{T,k} \\ h_T \\ -c_T \\ q_{T+1} \\ %\hat{\gamma}_{T+1,k}s_{T+1,k}
            -\rho\mathbf{1}\\ g_{T+1,k} - s_{T+1,k} \\ h_{T+1}  \\ r_{u_T^2}^1
        \end{bmatrix} = 0
    \end{aligned}
\end{equation*}
where $\Pi_T^{2} = [\nabla_{u_T^1} \pi_T^2,0]$
% where each row of the KKT condition represents: $\nabla_{u_t}L=0$, $\nabla_{u_t} (\hat{\gamma}_{T,k}g_{T}(x_t,u_t)-\frac{1}{t}\mathbf{1})=0$, $\nabla_{u_t}H=0$, $x_{t+1}=Ax_t + Bu_t$, $\nabla_{x_{T+1}}L=0$, $\nabla_{x_{T+1}}(\hat{\gamma}_{T+1,k}g(x_{T+1}))=0$, $\nabla_{x_{T+1}}H=0$, $\nabla_{x_t}(u_{t}^2 - \pi_t^2(x_t,u_t^1))$. 
At time $t = T-1$, the follower has the KKT condition:
% \begin{equation*}
%     \begin{aligned}
%         \begin{bmatrix}
%             E_t^{2} & W_t^2\\ N_{t+1} & M_{t+1} 
%         \end{bmatrix}
%     \end{aligned}
% \end{equation*}

\begin{equation*}\small
    W_t^2 = \begin{bmatrix}
        &0& 0 &0 & 0 & 0&0&0 \\
        % &0&0&0&0&0&0&0\\
        % &0&0&0&0&0&0&0\\
        % & 0 & 0 & 0&0&0&0 &0\\
        % &0  & 0 & 0&0&0&0&0\\
        &{S^{2\top}_{t+1}}&0 &-\hat{G}_{x_{t+1}}^{2\top} & -\hat{H}_{x_{t+1}}^{2\top} &0& A_{t+1}^\top & 0\\
        &  {\tilde{R}_{t+1}^2} &0& -\tilde{G}_{u_{t+1}^1}^{2\top} & -\tilde{H}_{u_{t+1}^1}^{2\top} &  0 & B_{t+1}^{1\top} & 0
    \end{bmatrix}
\end{equation*}
\begin{equation*}\small
    E_t^2 = \begin{bmatrix}
    {R_{t}^{2,2,2}} & 0& -G_{u_t^2}^{2\top} & -H_{u_t^2}^{2\top} & B_t^{2\top} & 0 &0  \\
            0 &\hat{\gamma}_{t}^2&\hat{s}_{t}^2 &0&0&0&0  \\
            G_{u_t^2}^2 &-I & 0 & 0 & 0 &0&0\\
            H_{u_t^2}^2 &0&0 & 0 & 0 & 0 & 0 \\
            -B_t^2&0 &0& 0 & 0 & 0 & I \\ 
            0&0 &0& 0 & -I & \pi_{t+1}^{1\top } & Q_{t+1}^2 \\
            % 0 & 0 &0&0&0& \hat{\gamma}^2_{t+1,k}G_{x_{t+1}}^2 & 0 & \hat{g}_{t+1,k}^2 & 0&0&0&0   \\
            0&0 &0& 0 & 0 & -I_{m_1} & {\tilde{S}^{2}_{x_{t+1}}}     
    \end{bmatrix}
\end{equation*}

\begin{equation*}\small
    \begin{aligned}
        &\left[\begin{array}{cc|c}
        & E_t^2 & W_t^2\\
            \hline 0&N_{t+1}&M_{t+1}          \end{array}\right] \cdot\begin{bmatrix}
            \Delta u_t^2 \\ \Delta s_t^2\\ \gamma_t^2 \\ \mu_t^2 \\ \lambda_t^2 \\ \eta_t^2 \\ \Delta x_{t+1} \\ z_{t+1}
        \end{bmatrix}  + \begin{bmatrix}
            {S_t^{2,2}} & {R_t^{2,2,1}} \\ 0 & 0 \\  G_{x_t}^2 & G_{u_t^1}^2  \\ H^2_{x_t} & H^2_{u_t^1} \\ -A_t & -B_t^1 \\ 0 & 0 \\ 0&0\\ 
            % 0 & 0 \\ 
            \hline 0 & 0
        \end{bmatrix}\begin{bmatrix}
            \Delta x_t \\ \Delta u_t^1
        \end{bmatrix}+ \begin{bmatrix}
        r_t^2 \\ %\hat{\gamma}_{t,k}^2g_{t,k}^2 
        - \rho\mathbf{1} \\ g_{t,k}^2 - s_{t,k}^2 \\ h^2_t \\ -c_t \\ q_{t+1}^2 \\
        % \hat{\gamma}^2_{t+1,k}g_{t+1,k}^2 - \frac{1}{t}\mathbf{1} \\ 
        { r_{u_{t+1}^1}^2} \\ \hline n_{t+1}
    \end{bmatrix}=0
    \end{aligned} 
\end{equation*}
We define $\tilde{R}_{t+1}^2 = \begin{bmatrix}
            R_{t+1}^{2,1,1}  R_{t+1}^{2,1,2}
        \end{bmatrix}$. We then consider the leader policy:
% where each line corresponds to: $\nabla_{u_t^2} L=0$, $H^2_t=0$, $x_{t+1}-Ax_t - Bu_t=0$, $\nabla_{x_{t+1}} L=0$, $\nabla_{u_{t+1}^1}L=0$.
% \begin{equation*}
%     \begin{aligned}
%         \tilde{R}_{t+1}^2 = \begin{bmatrix}
%             R_{t+1}^{2,1,1} & R_{t+1}^{2,1,2}
%         \end{bmatrix}
%     \end{aligned}
% \end{equation*}

% So, all the equality constraints are considered as $\lambda_t^i(-x_{t+1}+A x_t + Bu_t)$, $\eta_t^2 (\pi_{t+1}^1 x_{t+1} - u_{t+1}^1)$, and $\mu_t^2(-H^2_{x_t} x_t - H^2_{u_t^1}u_t^1 - H^2_{u_t^2}u_t^2-h^2_t )$.

\begin{equation*}\small
    E_t^1=\begin{bmatrix}
        {R_t} &0 & -\hat{G}_{u_t}^\top & -\hat{H}_{u_t}^{\top}& \hat{B}_t^\top & {0} &  {\Pi_t^{2\top}} & 0 \\
        0& \hat{\gamma}_{t,k} & \hat{s}_{t,k} &0&0&0&0&0\\
        G_{u_t} &-I &0 &0 &0 &0 &0 &0 \\
        H_{u_t} &0 & 0 & 0 & 0 & 0 & 0 & 0  \\
        -B_t&0 &0 & 0 & 0 & 0 & 0 & I_n   \\ 
        0 &0&0 & 0 & -I_{2n} & \Pi_{t+1}^\top &0 & Q_{t+1}  \\
        {0} &0&0 & 0 & 0 & -I_m & 0 & {\tilde{S}_{x_{t+1}}} \\
        {\tilde{R}_t^{12}} &0&-\tilde{G}_{u_t}^{12\top} & -\tilde{H}_{u_t}^{12\top} & \tilde{B}_t^{2\top} & 0 & -I_{m_2} & 0  \\
    \end{bmatrix}
\end{equation*}
\begin{equation*}\small
    W_t^1 = \begin{bmatrix}
        0&0&0&0&0&0\\
        {S_{u_{t+1}}} &0 & -\hat{G}_{x_{t+1}}^\top & -\hat{H}_{x_{t+1}}^\top  & \hat{A}_{t+1}^\top & 0 \\
        {\tilde{R}_{t+1}} &0 & -\tilde{G}_{u_{t+1}}^\top & -\tilde{H}_{u_{t+1}}^\top  & \tilde{B}_{t+1}^\top & 0 \\
        0 &0&0&0 & 0 &0 \\
    \end{bmatrix}
\end{equation*}

\begin{equation*}\small
    \begin{aligned}
        &\left[\begin{array}{c c  |  c }
             & E_t^1 & W_t^1\\
             \hline 0 & N_{t+1} & M_{t+1}
        \end{array}\right] \cdot  \begin{bmatrix}
            \Delta u_t \\ \Delta s_t\\ \gamma_t \\ \mu_t \\ \lambda_t \\ \eta_t \\ \psi_t^1 \\ \Delta x_{t+1} \\ z_{t+1}
        \end{bmatrix}   + \begin{bmatrix}
            {S_{x_t}} \\ 0 \\ G_{x_t} \\ H_{x_t} \\ -A_t \\ 0 \\0 \\ S_{t}^{12} \\ \hline 0
        \end{bmatrix}\Delta x_t +\begin{bmatrix}
            r_t \\ %\hat{\gamma}_{t,k}s_{t,k} 
            - \rho\mathbf{1} \\ g_{t,k} - s_{t,k} \\ h_t \\  -c_t \\ q_{t+1} \\ 
            % \hat{\gamma}_{t+1,k} g_{t+1,k}-\frac{1}{t}\mathbf{1} \\
            { \tilde{r}_{t+1}^2} \\{r_{u_t^2}^1} \\ \hline n_{t+1}
        \end{bmatrix} = 0
    \end{aligned}
\end{equation*}
% where each line corresponds to: $\nabla_{u_t^i} L^i=0$, $H_t=0$, $x_{t+1}-Ax_t - Bu_t=0$, $\nabla_{x_{t+1}} L^i=0$, $\nabla_{u_{t+1}^{-i}}L^i=0$, $\nabla_{u_t^2}L^1=0$. \\
We continue this construction process until $i=1$ and $t = 0$.
