# Supplementary material for: The computation of approximate feedback Stackelberg equilibria in multi-player nonlinear constrained dynamic games
Source: arXiv:2401.15745 source file (2025-04-02)
Supplement: Supplementary file 3 [file appendix_violating_strict_cvx_condition.tex]

\subsection{An Example violating Assumption~\ref{assumption:strict convex} but having feedback Stackelberg policies}\label{subsec:appendix existence of policy} Considering the following two-player game,
\begin{equation}
    \begin{aligned}
        \min_{u_t^1} &\  x_t - (u_t^1)^3 
        &\textrm{s.t. }x_{t+1}=x_t - (u_t^1)^2 - (u_t^2)^2 , u_t^1 \in [-\frac{1}{2},1] \\
        \min_{u_t^2} &\ (x_t)^3   
        &\textrm{s.t. }x_{t+1} = x_t - (u_t^1)^2 - (u_t^2)^2, u_t^2 \in [-\frac{1}{2},1]
    \end{aligned}
\end{equation}
and the terminal costs are $\ell_{T+1}^1:=x_{T+1}$ and $\ell_{T+1}^2:=(x_{T+1})^3$. The feedback Strategy is $\pi_t^1(x_t) = 1$, and $\pi_t^2(x_t,u_t^1)=1$.
